# Supplementary material for: Bayesian Parameterization of Continuum Battery Models from Featurized Electrochemical Measurements Considering Noise
Source: arXiv:2208.03289 ancillary file (2023-02-07)
Supplement: Supplementary file 1 [file SI.pdf]

# Supporting Information

## Bayesian Parameterization of Continuum Battery Models from Featurized Electrochemical Measurements Considering Noise

Yannick Kuhn\*

*German Aerospace Center, Pfaffenwaldring 38-40, 70569 Stuttgart, Germany and  
Helmholtz Institute Ulm, Helmholtzstraße 11, 89081 Ulm, Germany*

Hannes Wolf

*BASF SE, Carl-Bosch-Straße 38, 67056 Ludwigshafen am Rhein, Germany*

Arnulf Latz† and Birger Horstmann‡

*German Aerospace Center, Pfaffenwaldring 38-40, 70569 Stuttgart, Germany  
Helmholtz Institute Ulm, Helmholtzstraße 11, 89081 Ulm, Germany and  
Universität Ulm, Albert-Einstein-Allee 47, 89081 Ulm, Germany*

### SI-I. BATTERY MODEL BOUNDARY CONDITIONS

The natural boundary conditions, listed in Equation SI-1, basically enforce that no ions pass through the current collectors, enforce that the cell does not leak any electrolyte, and define the zero potential at the anode current collector. These boundary conditions result in zero-Neumann boundary conditions for  $c_e$  and  $\phi_e$  and a zero-Dirichlet boundary condition for  $\phi_{s,n}$ . Additionally, concentrations, fluxes, and potentials must be continuous at the boundaries between the electrodes and the separator. The coordinates  $x = 0$  and  $x = 1$  are assigned to the anode and cathode current collectors, respectively. The initial conditions are always assumed to be homogeneous across the cell since that is its equilibrium state.

$$i_{e,n} \Big|_{x=0} = 0, \quad (\text{SI-1.1})$$

$$i_{e,p} \Big|_{x=1} = 0, \quad (\text{SI-1.2})$$

$$N_{e,n} \Big|_{x=0} = 0, \quad (\text{SI-1.3})$$

$$N_{e,p} \Big|_{x=1} = 0, \quad (\text{SI-1.4})$$

$$\phi_{s,n} \Big|_{x=0} = 0. \quad (\text{SI-1.5})$$

The current-driving and coupling boundary conditions, listed in Equation SI-2 [1], match the potential gradient at the cathode current collector to the applied current, enforce symmetry at the particle centres, and apply the intercalation reaction current density to the outer boundaries of the particles. These boundary conditions are all Neumann boundary conditions for  $\phi_{s,p}$  and  $c_{s,k}$ . Additionally, the inner boundary conditions for  $\phi_{s,n}$  at  $x = L_n$  and  $\phi_{s,p}$  at  $x = 1 - L_p$  are zero-Neumann boundary conditions.

$$\partial_x \phi_{s,p} \Big|_{x=1} = -\frac{I}{\sigma_p \cdot (1 - \varepsilon_p)^{\beta_p}}, \quad (\text{SI-2.1})$$

$$\partial_{r_k} c_{s,k} \Big|_{r_k=0} = 0, \quad (\text{SI-2.2})$$

$$-a_k \gamma_k \frac{D_{s,k}(c_{s,k})}{C_k} \partial_{r_k} c_{s,k} \Big|_{r_k=1} = i_{se,k}. \quad (\text{SI-2.3})$$

### SI-II. EXPONENTIAL FAMILIES

The general form of an exponential family is described by Equation SI-3. For example, Gaussian distributions and other common distributions with non-vanishing probabilities are elements of exponential families.

$$P_{\lambda}(\theta) \propto \exp(\lambda \cdot \mathbf{t}(\theta)). \quad (\text{SI-3})$$

Here,  $\mathbf{t} : \mathbb{R}^m \mapsto \mathbb{R}^n$  is any (vector) function that is integrable.  $\mathbf{t}$  defines its exponential family uniquely. Distinct distributions in an exponential family are labelled by their “natural parameters”  $\lambda \in \mathbb{R}^n$ . For example, the mean  $\mu$  and covariance  $\Sigma$  of a Gaussian distribution may be encoded in such a vector  $\lambda$ ,

$$\lambda = \left( \mathbf{r}, -\frac{1}{2}\mathbf{Q} \right), \mathbf{r} := \Sigma^{-1}\mu, \mathbf{Q} := \Sigma^{-1}. \quad (\text{SI-4})$$

The moment-matching aspect of Expectation Propagation is verified for exponential families by differentiation, as shown in Equation SI-5 [2].

$$\frac{d}{d\lambda} KL(\pi || P_{\lambda}) = \mathbb{E}_{P_{\lambda}}(\mathbf{t}) - \int_{\Theta} \mathbf{t}(\theta) \pi(\theta) d\theta. \quad (\text{SI-5})$$

### SI-III. DAMPENING IN EXPECTATION PROPAGATION

With a dampening parameter  $\alpha \in ]0, 1[$ , dampening is introduced to Expectation Propagation (EP) by linearly interpolating between  $P(\theta|y)$  prior to each site update and  $P_{+i}(\theta|y)$

\* yannick.kuhn@dlr.de

† arnulf.latz@dlr.de

‡ birger.horstmann@dlr.de

in terms of their so-called “natural parameters”  $\lambda$ . [2] Please see the previous Section SI-II for details about  $\lambda$ .

In Expectation Propagation,  $\lambda$  is factorized into a sum of  $\lambda_i$  for each Likelihood site. Let  $\lambda_{+i}$  denote the Pseudo-Posterior,  $\lambda$  the current Posterior before each site update,  $\lambda_{\text{new}}$  the current Posterior after each site update and  $\lambda_{i,\text{new}}$  the Likelihood site after its update. Without dampening, the EP update step looks like this:

$$\lambda_{\text{new}} := \lambda_{+i}, \lambda_{i,\text{new}} := \lambda_i + \lambda_{+i} - \lambda. \quad (\text{SI-6})$$

With the convention that  $\alpha = 0$  refers to zero dampening and  $\alpha = 1$  refers to total dampening, i.e., no update, the EP update step with dampening looks like this:

$$\lambda_{\text{new}} := (1 - \alpha)\lambda_{+i} + \alpha\lambda, \lambda_{i,\text{new}} := \lambda_i + (1 - \alpha)(\lambda_{+i} - \lambda). \quad (\text{SI-7})$$

#### SI-IV. DERIVATION OF THE SURROGATE IN BOLFI

The model parameter samples  $\theta_k$  and the deviations between simulation and experiment  $\log(\|y_i(\theta_k) - y_i^*\|)$  constitute the data that BOLFI trains a surrogate function on. Here,  $y_i^*$  is the current feature of the experimental data and  $y_i(\theta_k)$  is the simulated feature for the parameter set  $\theta_k$ . We now denote the collection of all model-simulation comparisons as  $\Delta_K$ .

$$\Delta_K := \left[ \log(\|y_i(\theta_k) - y_i^*\|) \right]_{k=1}^K. \quad (\text{SI-8})$$

$K$  refers to the total number of samples taken up to any point in the algorithm. Square brackets  $[\dots]_{k=1}^K$  denote a vector of length  $K$ , while square brackets with two indices  $[\dots]_{k,\ell=1}^K$  will denote a square matrix with  $K$  rows and  $K$  columns.

In the next step, we assume that the model-simulation comparisons  $\Delta_K$  follow a Gaussian Process,

$$\Delta_K \sim \mathcal{N}(\mathbf{m}_K, \mathbf{K}_K). \quad (\text{SI-9})$$

This Gaussian Process is the Gaussian distribution  $\mathcal{N}$  defined by sample evaluations of the mean  $\mathbf{m}_K$  and covariance matrix  $\mathbf{K}_K$ ,

$$\mathbf{m}_K := [\tilde{\mu}_K(\theta_k)]_{k=1}^K, \quad (\text{SI-10.1})$$

$$\mathbf{K}_K := [\tilde{v}_K(\theta_k, \theta_\ell)]_{k,\ell=1}^K + \sigma^2 \mathbb{1}. \quad (\text{SI-10.2})$$

The mean  $\tilde{\mu}_K$  and variance  $\tilde{v}_K$  functions are assumed as a parabolic function plus noise,

$$\tilde{\mu}_K(\theta) := \sum_{j=1}^d (a_j \theta_j^2 + b_j \theta_j + c), \quad (\text{SI-11.1})$$

$$\tilde{v}_K(\theta, \vartheta) := \sigma_f^2 \exp \left( \sum_{j=1}^d \frac{(\theta_j - \vartheta_j)^2}{\lambda_j^2} \right), \quad (\text{SI-11.2})$$

and updated slowly with every acquired sample by adjusting  $a_j \geq 0$ ,  $b_j$ ,  $c$ ,  $\sigma_f^2 > 0$ ,  $\lambda_j$ , and  $\sigma^2 > 0$ . [3]  $\tilde{\mu}_K$  and  $\tilde{v}_K$  constitute a Prior for the model-simulation discrepancy function  $\log(\|y_i(\cdot) - y_i^*\|)$ .

BOLFI now calculates a Posterior to the model-simulation discrepancy function  $\log(\|y_i(\cdot) - y_i^*\|)$ ,

$$\log(\|y_i(\theta) - y_i^*\|) \sim \mathcal{N}(\mu_K(\theta), v_K(\theta) + \sigma^2), \quad (\text{SI-12})$$

where  $\mu_K$  and  $v_K$  are constantly updated with the generated samples by a Kalman-like filter [3],

$$\mathbf{k}_K(\theta) := \left[ \tilde{v}_K(\theta, \theta_k) \right]_{k=1}^K, \quad (\text{SI-13.1})$$

$$\mu_K(\theta) := \tilde{\mu}_K(\theta) + \mathbf{k}_K(\theta)^t \mathbf{K}_K^{-1} (\Delta_K - \mathbf{m}_K), \quad (\text{SI-13.2})$$

$$v_K(\theta) := \tilde{v}_K(\theta, \theta) - \mathbf{k}_K(\theta)^t \mathbf{K}_K^{-1} \mathbf{k}_K(\theta). \quad (\text{SI-13.3})$$

Please note that the states of this Kalman-like Filter do not represent time points in a measurement but sample points in the optimization process.

#### SI-V. VALIDATION OF EP-BOLFI PERFORMANCE

We recapitulate the estimation task we use for validation. Our reference for state-of-the-art automated battery model parameterization is the work of Aitio et al. [4]. They create two types of synthetic data with an SPMe model, multimodal sinusoidal excitations at eleven SOC's denoted “excitation-point case” and a discharge with a superimposed small unimodal sinusoidal excitation denoted “wide-excursion case”. Aitio et al. fit five parameters with an MCMC algorithm: the electrolyte  $D_e^*$  and solid diffusivities  $D_{s,n}^*$ ,  $D_{s,p}^*$ , the cation transference number  $t_+$ , and the variance of the white noise superimposed on the synthetic measurement. In the wide-excursion case, MCMC fits the parameters nicely. However, the MCMC algorithm finds a wide range of inconsistent values in the excitation-point case [4].

The priors in Aitio et al. are Gamma distributions for the diffusivities and a Beta distribution for the cation transference number. We approximate the Gamma distributions with log-normal distributions and the Beta distribution with a normal distribution. EP-BOLFI does not support improper priors. Thus, we replace the infinite uniform distribution for the measurement noise with a log-normal distribution. Further details and the parameter set we use can be found in the accompanying GitHub repository.

The features we use in EP-BOLFI for the wide-excursion case are  $L^2$ -distances of voltage curve segments corresponding to the initial electrolyte relaxation, the first full sine wave after that, the last full sine wave, and the rest of the voltage curve in-between.

In Table SI-I we show the results for the validation of EP-BOLFI against the excitation-point case of Aitio et al. [4] at excitation point 11. With MCMC, one parameter remained highly uncertain, while EP-BOLFI got to within 20% of the true values. We conclude that EP-BOLFI is at least as stable to measurement noise as MCMC and prospectively more so while also converging faster.

Table SI-II is the equivalent to Table 3 in Aitio et al. [4], where we compare MCMC and EP-BOLFI on all estimation cases stated there. The values for MCMC were obtained

TABLE SI-I. Performance comparison between MCMC [4] and EP-BOLFI for a multiharmonic excitation, namely excitation-point case 11.

| parameter                                   | true value | initial standard deviation | Aitio et al. (MCMC), 100 000 simulations | EP-BOLFI 2080 simulations | EP-BOLFI 4160 simulations | EP-BOLFI 6240 simulations |
|---------------------------------------------|------------|----------------------------|------------------------------------------|---------------------------|---------------------------|---------------------------|
| $D_e^* / 10^{-10} \text{ m}^2/\text{s}$     | 2.8        | 1.54                       | $1.19 \pm 1.01$                          | $3.42 \pm 2.07$           | $3.31 \pm 1.70$           | $3.23 \pm 1.41$           |
| $t_+ / -$                                   | 0.40       | 0.156                      | $0.43 \pm 0.03$                          | $0.40 \pm 0.06$           | $0.40 \pm 0.05$           | $0.40 \pm 0.05$           |
| $D_{s,n}^* / 10^{-14} \text{ m}^2/\text{s}$ | 3.9        | 1.39                       | $3.83 \pm 0.03$                          | $4.23 \pm 2.12$           | $3.99 \pm 1.56$           | $4.07 \pm 1.38$           |
| $D_{s,p}^* / 10^{-13} \text{ m}^2/\text{s}$ | 1.0        | 1.98                       | $14.77 \pm 14.28$                        | $1.46 \pm 1.58$           | $1.27 \pm 1.14$           | $1.21 \pm 0.98$           |
| $\sigma^2 / 10^{-9} \text{ V}^2$            | 1.6        | 1.17                       | $1.61 \pm 0.11$                          | $1.67 \pm 0.90$           | $1.57 \pm 0.68$           | $1.61 \pm 0.67$           |

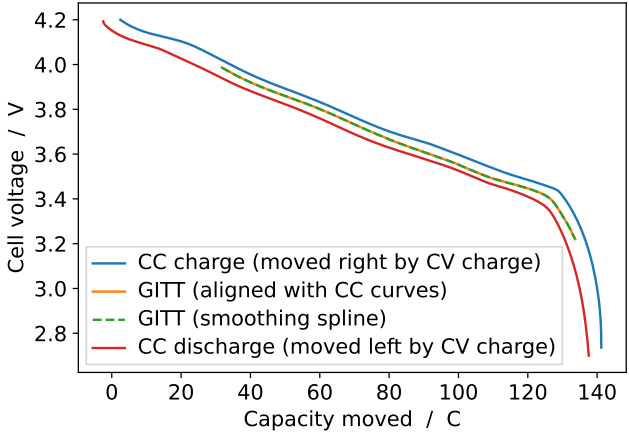

FIG. SI-1. The CC-curves at 1/3 C and the GITT measurement of the full cell for the OCV identification.

with 100 000 simulations, while those for EP-BOLFI are obtained with 6240 simulations. We give the comparison with posterior mean  $\theta$  and posterior standard deviation  $\sigma$ , just as Aitio et al. did. We also performed an additional experiment, collating the four excitation points 1, 3, 6, and 11 with the smallest uncertainties. This experiment shows that EP can easily incorporate an arbitrary number of features.

The Gamma distributions for  $D_{s,n}^*$ ,  $D_{s,p}^*$  and  $D_e^*$  with MCMC may be compared to their respective log-normal distributions with EP-BOLFI as follows. For  $\sigma \ll \theta$ , both types of distributions are roughly symmetrical with mode close to their mean. For  $\sigma \approx \theta$ , both types of distributions are asymmetrical and wide but still roughly comparable. For  $\sigma > \theta$ , both types of distributions indicate that the corresponding parameter was not identified. Scaling the parameter by a constant scales mean and standard deviation by the same constant for both types of distributions.

#### SI-VI. DIFFERENCE QUOTIENT OF ONE OCV FROM GITT AND CC-CV

Given  $U_n$ , we determine the SOCS  $\text{SOC}_p$  and  $\text{SOC}_n$  of positive and negative electrode, respectively, as functions of an arbitrary cell SOC  $s$ . We do so by analyzing the stoichiometric drift  $c_{s,k}(t, x, r_k = 1) - \int c_{s,k}(t, x, r_k) dr_k$ . While the first term gives the electrode SOC as it appears in the voltage curve measured during CC, the second term gives

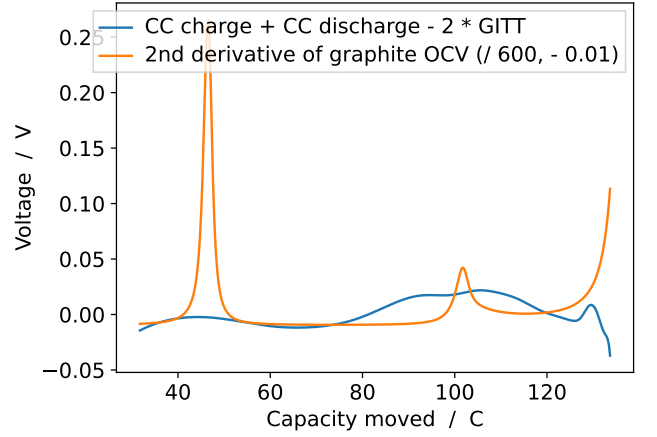

FIG. SI-2. The second derivative of graphite OCV from literature [5], aligned with the processed data from Figure SI-1. The hills are smoothed out due to the coarse difference quotient. We used the peaks for alignment.

the electrode SOC as it would be measured with coulombic counting. If we can shift the measured voltage curves by the stoichiometric drift of one electrode, we can build a difference quotient for the other electrode with charge, discharge and GITT data.

Figure SI-1 shows the data we will use for this: a GITT measurement and one CC-CV cycle of the full cell. The charge and discharge curves are shifted by the charge moved during the CV step in opposing directions. The GITT OCV data itself is obtained as the exponential decay limit of each GITT pulse. Figure SI-2 shows the approximated second derivative of  $U_n$ .

Motivated by the SPM<sub>e</sub>(S) [1], we assume that the deviation between bulk SOC and surface SOC is constant across each electrode and that the electrolyte only acts as a resistor. For ease of calculation,  $D_{s,k}(\cdot)$  will be constants; without loss of generality, let  $D_{s,k}(\cdot) \equiv 1$ . The SPM<sub>e</sub>(S) equations we need to solve are:

$$C_k \partial_t c_{s,k}^{(0)} = r_k^{-2} \partial_{r_k} \left( r_k^2 \partial_{r_k} c_{s,k}^{(0)} \right), \quad (\text{SI-14})$$

$$\partial_{r_k} c_{s,k}^{(0)} \Big|_{r_k=0} = 0, \quad (\text{SI-15})$$

$$\partial_{r_k} c_{s,k}^{(0)} \Big|_{r_k=1} = \mp \frac{C_k I}{a_k \gamma_k L_k}. \quad (\text{SI-16})$$

We choose the integration constant such that  $\int c_{s,k}(t =$

TABLE SI-II. Stability comparison between MCMC [4] (100 000 simulations) and EP-BOLFI (6240 simulations).  $\theta$  are posterior means and  $\sigma$  are posterior standard deviations.

| Parameter            |                            | Excitation Point |       |       |       |      |      |       |      |      |       |       | Wide Excursion       | Collation      |
|----------------------|----------------------------|------------------|-------|-------|-------|------|------|-------|------|------|-------|-------|----------------------|----------------|
|                      |                            | 1                | 2     | 3     | 4     | 5    | 6    | 7     | 8    | 9    | 10    | 11    |                      | 1 & 3 & 6 & 11 |
|                      | $c_{s,n}$                  | 0.80             | 0.73  | 0.67  | 0.61  | 0.55 | 0.49 | 0.43  | 0.37 | 0.31 | 0.25  | 0.19  |                      |                |
|                      | $c_{s,p}$                  | 0.51             | 0.55  | 0.59  | 0.62  | 0.66 | 0.69 | 0.73  | 0.76 | 0.80 | 0.83  | 0.87  |                      |                |
| $D_{s,n}^*/10^{-14}$ | $\theta_{\text{EP-BOLFI}}$ | 4.13             | 3.93  | 3.99  | 4.39  | 3.79 | 3.93 | 4.16  | 4.51 | 4.49 | 4.01  | 4.07  | 3.90                 | 3.29           |
|                      | $\sigma_{\text{EP-BOLFI}}$ | 1.76             | 1.51  | 1.64  | 1.87  | 1.63 | 1.51 | 1.64  | 2.06 | 1.89 | 1.67  | 1.38  | $44.2 \cdot 10^{-4}$ | 0.80           |
|                      | $\theta_{\text{MCMC}}$     | 13.98            | 19.47 | 13.24 | 14.81 | 3.27 | 3.39 | 12.74 | 5.92 | 5.59 | 3.73  | 3.83  | 3.90                 |                |
|                      | $\sigma_{\text{MCMC}}$     | 10.55            | 14.64 | 16.48 | 14.41 | 1.27 | 0.27 | 11.64 | 5.01 | 4.88 | 0.08  | 0.03  | $5.05 \cdot 10^{-4}$ |                |
| $D_{s,p}^*/10^{-13}$ | $\theta_{\text{EP-BOLFI}}$ | 1.25             | 1.31  | 1.23  | 1.34  | 1.62 | 1.26 | 1.25  | 1.31 | 1.25 | 1.28  | 1.21  | 1.00                 | 1.03           |
|                      | $\sigma_{\text{EP-BOLFI}}$ | 0.83             | 0.87  | 0.91  | 0.97  | 1.37 | 0.87 | 1.01  | 0.93 | 0.91 | 1.02  | 0.98  | $45.4 \cdot 10^{-4}$ | 0.66           |
|                      | $\theta_{\text{MCMC}}$     | 0.90             | 0.98  | 1.01  | 0.98  | 1.36 | 2.72 | 0.91  | 2.28 | 2.17 | 22.41 | 14.77 | 1.00                 |                |
|                      | $\sigma_{\text{MCMC}}$     | 0.12             | 0.02  | 0.08  | 0.03  | 0.42 | 1.58 | 0.40  | 2.24 | 2.09 | 25.09 | 14.28 | $1.70 \cdot 10^{-4}$ |                |
| $D_e^*/10^{-10}$     | $\theta_{\text{EP-BOLFI}}$ | 3.06             | 3.54  | 3.30  | 3.21  | 4.28 | 3.41 | 3.28  | 2.90 | 2.98 | 3.41  | 3.23  | 2.80                 | 5.15           |
|                      | $\sigma_{\text{EP-BOLFI}}$ | 1.46             | 1.94  | 1.65  | 1.88  | 2.35 | 1.72 | 1.78  | 1.51 | 1.38 | 1.79  | 1.42  | $23.7 \cdot 10^{-3}$ | 2.17           |
|                      | $\theta_{\text{MCMC}}$     | 2.43             | 5.51  | 5.34  | 4.04  | 2.73 | 4.76 | 2.49  | 3.07 | 0.98 | 4.69  | 1.19  | 2.80                 |                |
|                      | $\sigma_{\text{MCMC}}$     | 1.29             | 1.79  | 1.74  | 1.59  | 1.43 | 1.68 | 1.41  | 1.40 | 0.85 | 2.20  | 1.01  | $6.61 \cdot 10^{-3}$ |                |
| $t_+$                | $\theta_{\text{EP-BOLFI}}$ | 0.40             | 0.40  | 0.40  | 0.41  | 0.38 | 0.40 | 0.39  | 0.40 | 0.40 | 0.40  | 0.40  | 0.40                 | 0.35           |
|                      | $\sigma_{\text{EP-BOLFI}}$ | 0.06             | 0.06  | 0.04  | 0.05  | 0.06 | 0.05 | 0.05  | 0.05 | 0.06 | 0.04  | 0.05  | $30.9 \cdot 10^{-4}$ | 0.03           |
|                      | $\theta_{\text{MCMC}}$     | 0.41             | 0.36  | 0.37  | 0.38  | 0.42 | 0.36 | 0.43  | 0.36 | 0.45 | 0.40  | 0.43  | 0.40                 |                |
|                      | $\sigma_{\text{MCMC}}$     | 0.03             | 0.03  | 0.03  | 0.03  | 0.03 | 0.03 | 0.03  | 0.03 | 0.02 | 0.04  | 0.03  | $8.32 \cdot 10^{-4}$ |                |
| $\sigma^2/10^{-9}$   | $\theta_{\text{EP-BOLFI}}$ | 1.49             | 1.63  | 1.53  | 1.49  | 1.58 | 1.47 | 1.54  | 1.58 | 1.53 | 1.53  | 1.61  | 1.66                 | 0.30           |
|                      | $\sigma_{\text{EP-BOLFI}}$ | 0.63             | 0.76  | 0.60  | 0.60  | 0.64 | 0.48 | 0.66  | 0.59 | 0.61 | 0.67  | 0.67  | 0.09                 | 0.11           |
|                      | $\theta_{\text{MCMC}}$     | 1.60             | 1.59  | 1.60  | 1.60  | 1.61 | 1.59 | 1.61  | 1.61 | 1.58 | 1.59  | 1.61  | 1.39                 |                |
|                      | $\sigma_{\text{MCMC}}$     | 0.11             | 0.11  | 0.11  | 0.11  | 0.11 | 0.11 | 0.11  | 0.11 | 0.11 | 0.11  | 0.11  | 3.45                 |                |

$$0, r_k) dr_k = c_{s,k,0}:$$

$$c_{s,k}(t, r_k) = c_{s,k,0} \pm \frac{3C_k I}{10a_k \gamma_k L_k} \mp \frac{3I}{a_k \gamma_k L_k} \mp \frac{C_k I}{2a_k \gamma_k L_k} r_k^2. \quad (\text{SI-17})$$

We now have analytical expressions for charge  $C$  and discharge  $D$  terminal voltage curves. For simplicity, let  $\tilde{\eta}_k$  be a catch-all term for overpotentials dependent on surface SOC and  $R$  be a catch-all term for current-dependent overpotentials.  $\Delta c_{s,k}$  is the unknown current-dependent constant denoting the deviation between bulk and surface SOC.

$$C(s) = U_p(\text{SOC}_p(s) - \Delta c_{s,p}) - U_n(\text{SOC}_n(s) + \Delta c_{s,n}) \quad (\text{SI-18})$$

$$+ R + \tilde{\eta}_p(\text{SOC}_p(s) - \Delta c_{s,p}) + \tilde{\eta}_n(\text{SOC}_n(s) + \Delta c_{s,n}) \quad (\text{SI-19})$$

$$D(s) = U_p(\text{SOC}_p(s) + \Delta c_{s,p}) - U_n(\text{SOC}_n(s) - \Delta c_{s,n}) \quad (\text{SI-20})$$

$$- R - \tilde{\eta}_p(\text{SOC}_p(s) + \Delta c_{s,p}) - \tilde{\eta}_n(\text{SOC}_n(s) - \Delta c_{s,n}) \quad (\text{SI-21})$$

While  $\Delta c_{s,k}$  could be calculated analytically, we may not know the relevant parameters. Instead, we will assume that  $\Delta c_{s,p} \gg \Delta c_{s,n}$ , i.e., the transport limitation inside the positive electrode active material dominates the CV step. Thus, we can displace  $C$  and  $D$  by the charge  $C_{CV}$  and assume that this cancels out  $\Delta c_{s,p}$ . This step involves the linear transformation factor between  $s$  and  $\text{SOC}_p$ , so  $C_{CV}$  and  $\Delta c_{s,p}$  may be different. Likewise, a displacement of  $\text{SOC}_n$  occurs, which we label  $\delta$ .

$$\Delta U(s) := C(s + C_{CV}) - D(s - C_{CV}) \quad (\text{SI-22})$$

$$\approx 2R + 2\tilde{\eta}_p(\text{SOC}_p(s)) \quad (\text{SI-23})$$

$$+ \tilde{\eta}_n(\text{SOC}_n(s) + \delta) + \tilde{\eta}_n(\text{SOC}_n(s) - \delta) \quad (\text{SI-24})$$

$$+ U_n(\text{SOC}_n(s) + \delta) - U_n(\text{SOC}_n(s) - \delta), \quad (\text{SI-25})$$

$$\Delta^2 U(s) := C(s + C_{CV}) + D(s - C_{CV}) \quad (\text{SI-26})$$

$$- 2(U_p(\text{SOC}_p(s)) - U_n(\text{SOC}_n(s))) \quad (\text{SI-27})$$

$$\approx - U_n(\text{SOC}_n(s) + \delta) + 2U_n(\text{SOC}_n(s)) \quad (\text{SI-28})$$

$$- U_n(\text{SOC}_n(s) - \delta) \quad (\text{SI-29})$$

$$- \tilde{\eta}_n(\text{SOC}_n(s) + \delta) + \tilde{\eta}_n(\text{SOC}_n(s) - \delta). \quad (\text{SI-30})$$

Note that the definition of  $\Delta^2 U$  contains  $U_p$ , which we do not know. But we do know  $U_p(\text{SOC}_p(s)) - U_n(\text{SOC}_n(s))$ , since that is precisely the GITT measurement. So in effect, we added the two CC curves, displaced by the CV step, and subtracted the GITT curve from each. The result approximates a difference quotient for the second derivative of  $U_n$  without the denominator  $\delta^2$ . The other terms are a difference quotient for the first derivative of  $\tilde{\eta}_n$  without the denominator  $2\delta$ . While  $\delta^2 < 2\delta$ , the terms for  $U_n$  should still dominate  $\Delta^2 U$ , since the overpotential for the negative electrode usually is much smaller than  $U_n$ . We choose  $\Delta^2 U$  over  $\Delta U$  for further analysis since the non- $U_n$  terms do not even approximately cancel out in  $\Delta U$ . Still,  $\Delta^2 U$  is only an approximation to a smoothed-out second derivative of  $U_n$ . We match the peaks

of  $U_n''$  to the hills of  $\Delta^2 U$  by adjusting  $\text{SOC}_n(\cdot)$  and obtain  $\text{SOC}_n(\cdot)$  this way.

### SI-VII. MOTIVATION OF THE FEATURES IN THE GITT EXPERIMENT

Chien et al. [6] present in their Supporting Information an analytic solution to the diffusion equation for the electrode particles in an SPM model. When the current is switched from zero to a constant value  $I^*$ , the particle surface concentration takes this form:

$$c_{s,k}^*(t^*, R_k^*) = c_{s,k}^*(0, R_k^*) - \frac{I^* R_k^*}{F A^* D_{s,k}^*} f\left(\frac{D_{s,k}^* t^*}{R_k^{*2}}\right), \quad (\text{SI-31})$$

$$f(y) := 3y + 0.2 - 2 \sum_{m=1}^{\infty} \frac{1}{\alpha_m^2} \exp(-\alpha_m^2 y). \quad (\text{SI-32})$$

Chien et al. obtain a similar solution for a current that is switched off. Here,  $\alpha_m$  are the positive roots of  $\alpha \mapsto \tan(\alpha) - \alpha$ . The helper function  $f$  may be approximated within 5% error by:

$$f(y) \approx \begin{cases} \frac{2}{\sqrt{\pi}} \sqrt{y}, & y < 0.0032 \\ 3y + 0.2, & y > 1.27 \end{cases}. \quad (\text{SI-33})$$

The term  $3y$  represents the long-term change in the bulk SOC proportional to the applied current. Since we subtract the OCV from the measurement and keep SOC-dependent parameters locally constant, that linear term will not affect the overpotential. What remains is a different approximation for large  $y > 1.27$ :

$$0.2 - 2 \exp(-\alpha_1^2 x). \quad (\text{SI-34})$$

Therefore, we expect the electrode with the faster kinetics to dominate the initial square root term, while the other should dominate the exponential decay towards equilibrium. The electrolyte properties also affect these features in the simulations, but the square root fits and the exponential fit still describe the data well.

The analytical formula for GITT and ICI is the same [6]:

$$D_{s,p}^* = \frac{4}{\pi} \left( \frac{I^*}{F A^*} \frac{\frac{dc_{s,p}^*}{dt^*} \big|_{t^*=R_p^*}}{\frac{dU^*(t^*)}{d\sqrt{t^*}}} \right)^2. \quad (\text{SI-35})$$

### SI-VIII. JOINT RESISTANCE OF BOTH EXCHANGE-CURRENT DENSITIES

Figure SI-3 showcases the resistance the two exchange-current densities contribute in the Single-Particle Model [1]

with linearized overpotential term. The corresponding term is

$$\frac{R^* T^*}{F^* A^*} \left( \frac{1}{z_n \frac{\gamma_n}{C_{r,n}} i_{se,n,0}^* L_n} + \frac{1}{z_p \frac{\gamma_p}{C_{r,p}} i_{se,p,0}^* L_p} \right). \quad (\text{SI-36})$$

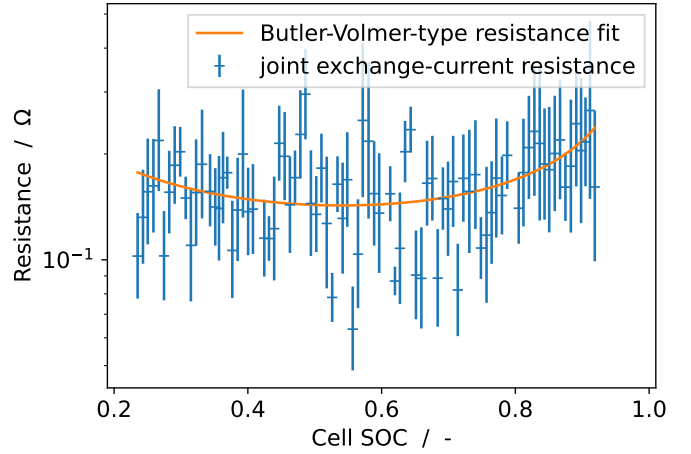

FIG. SI-3. The joint resistance of both exchange-current densities. The error bars consider the highest and lowest values of the two exchange-current densities. The formula we use is in Equation SI-36.

### SI-IX. SENSITIVITY OF THE DFN MODEL TO GITT DATA

In the following, we analyze the sensitivity of measurement features to estimated parameters by exploring the on standard deviation boundaries of the fitted logarithmic model parameters in SI-4. We assume a linearized sensitivity within these boundaries. The formula we use in SI-4 for each logarithmic fit parameter  $\theta_j$  to each feature  $y_i$  is

$$\frac{\Delta y_i}{y_i} = \text{sensitivity}_{ij} \cdot \frac{\Delta \theta_j}{\theta_j}. \quad (\text{SI-37})$$

We observe the following relations. Every parameter has a major effect on the exponential relaxation time, but we also saw in the main text that this feature is unreliable.  $i_{se,n,0}^*$  and  $i_{se,p,0}^*$  have a major effect on the exponential relaxation time and the ohmic voltage drop, but only on them.  $D_{s,n}^*$  and  $D_{s,p}^*$  affect all features but the ohmic voltage drop.

### SI-X. CHECKLIST TO REPORT THEORETICAL BATTERY STUDIES

In Table SI-III we provide the “minimal information set” as it is suggested by Mistry et al. [7].

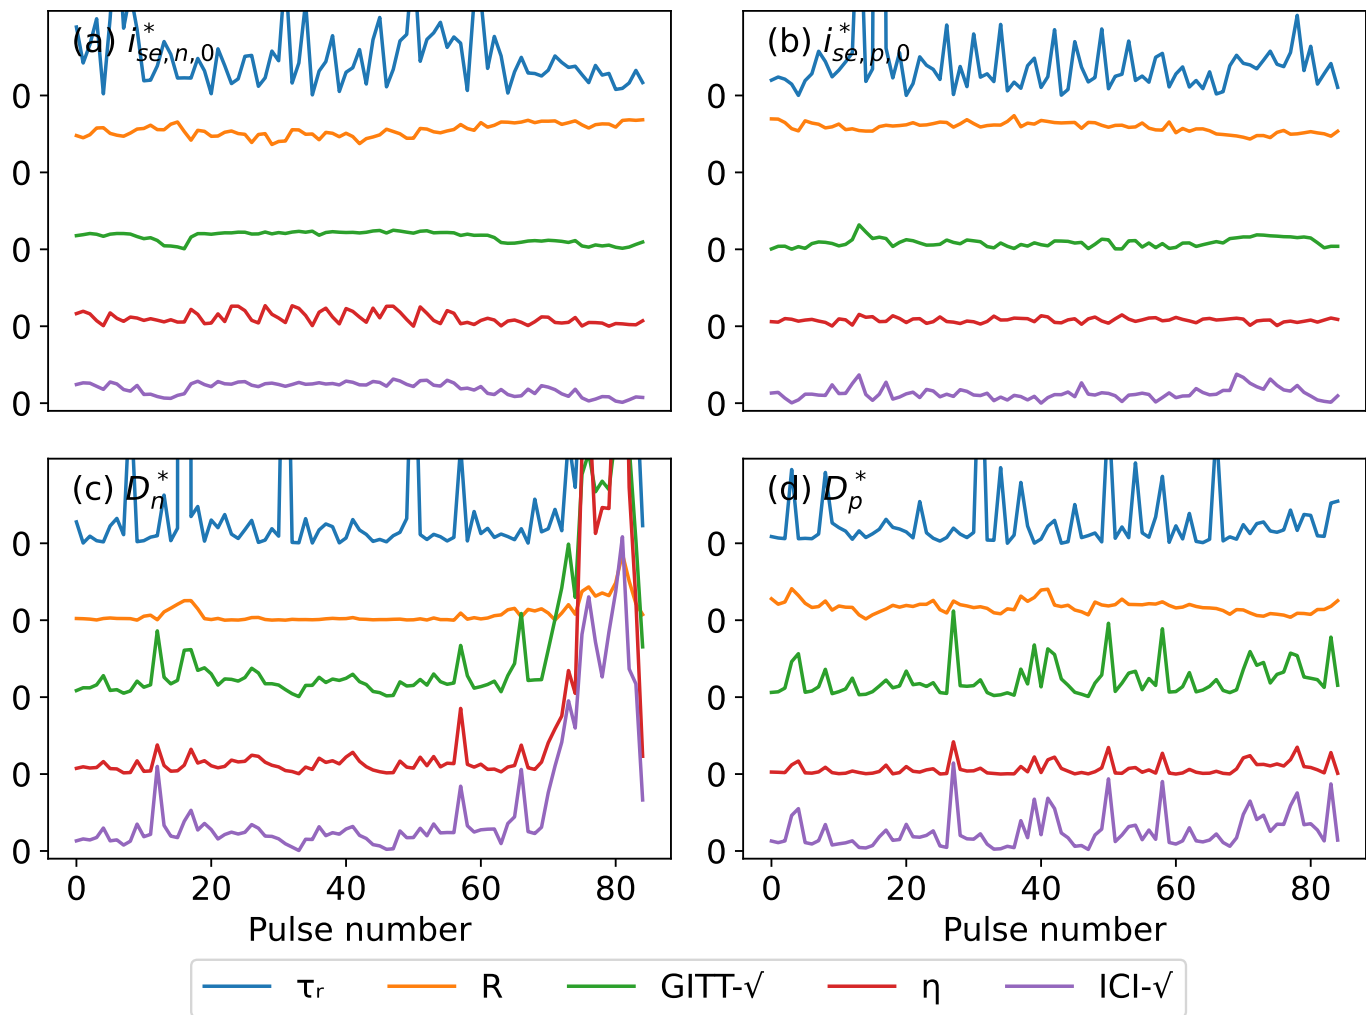

FIG. SI-4. The sensitivities of the five fitted features to the individual fit parameters within their one standard deviation intervals.  $i_{se,n,0}^*$  and  $i_{se,p,0}^*$  are the negative and positive electrode exchange-current densities, respectively, and  $D_{s,n}^*$  and  $D_{s,p}^*$  are the negative and positive electrode solid diffusivities, respectively. This Figure is calculated with the formula in SI-37. The abridged legend reads as follows:  $\tau_r$  is the exponential relaxation time,  $R$  is the ohmic voltage drop,  $GITT - \sqrt{\phantom{x}}$  is the GITT square root slope,  $\eta$  is the concentration overpotential, and  $ICI - \sqrt{\phantom{x}}$  is the ICI square root slope.

- 
- [1] S. G. Marquis, V. Sulzer, R. Timms, C. P. Please, S. J. Chapman, *J. Electrochem. Soc.* **2019**, 166, A3693.
- [2] S. Barthelmé, N. Chopin, V. Cottet, *Handbook of Approximate Bayesian Computation*, Chapman and Hall/CRC, 1st edition **2018**.
- [3] M. U. Gutmann, J. Corander, *J. Mach. Learn. Res.* **2016**, 17, 1.
- [4] A. Aitio, S. G. Marquis, P. Ascencio, D. Howey, *IFAC-PapersOnLine* **2020**, 53, 12497.
- [5] C. R. Birkel, E. McTurk, M. R. Roberts, P. G. Bruce, D. A. Howey, *J. Electrochem. Soc.* **2015**, 162, A2271.
- [6] Y.-C. Chien, H. Liu, A. S. Menon, W. R. Brant, D. Brandell, M. J. Lacey, *ChemRxiv* **2021**, pages 1–8.
- [7] A. Mistry, A. Verma, S. Sripad, R. Ciez, V. Sulzer, F. B. Planella, R. Timms, Y. Zhang, R. Kurchin, P. Dechent, W. Li, S. Greenbank, Z. Ahmad, D. Krishnamurthy, A. M. F. Jr., K. Tenny, P. Patel, D. J. Robles, P. Gasper, A. Colclasure, A. Baskin, C. D. Scown, V. R. Subramanian, E. Khoo, S. Allu, D. Howey, S. DeCaluwe, S. A. Roberts, V. Viswanathan, *ACS Energy Lett.* **2021**, 6, 3831.

TABLE SI-III. Minimal information set to enable verifiable theoretical battery research as suggested by [7]. \*I verify that this form is completed accurately in agreement with all co-authors, to the best of my knowledge. †Y  $\equiv$  the question is answered completely. Discuss any N or NA response in “Remarks”.

|                                                                                                                                                                              |                                                                                                                                                                                                                                                                                                                                                                                                                                                                                                                                                                                                                     |              |
|------------------------------------------------------------------------------------------------------------------------------------------------------------------------------|---------------------------------------------------------------------------------------------------------------------------------------------------------------------------------------------------------------------------------------------------------------------------------------------------------------------------------------------------------------------------------------------------------------------------------------------------------------------------------------------------------------------------------------------------------------------------------------------------------------------|--------------|
| Manuscript title: EP-BOLFI: Measurement-Noise-Aware Parameterization of Continuum Battery Models<br>from Electrochemical Measurements Applied to Full-Cell GITT Measurements |                                                                                                                                                                                                                                                                                                                                                                                                                                                                                                                                                                                                                     |              |
| Submitting author*:                                                                                                                                                          |                                                                                                                                                                                                                                                                                                                                                                                                                                                                                                                                                                                                                     | Yannick Kuhn |
| #                                                                                                                                                                            | Question                                                                                                                                                                                                                                                                                                                                                                                                                                                                                                                                                                                                            | Y/N/NA†      |
| 1                                                                                                                                                                            | Have you provided all assumptions, theory, governing equations, initial and boundary conditions, material properties (e.g., open-circuit potential) with appropriate precision and literature sources, constant states (e.g., temperature), etc.?<br><b>Remarks:</b>                                                                                                                                                                                                                                                                                                                                                | Y            |
| 2                                                                                                                                                                            | If the calculations have a probabilistic component (e.g., Monte Carlo, initial configuration in Molecular Dynamics, etc.), did you provide statistics (mean, standard deviation, confidence interval, etc.) from multiple ( $\geq 3$ ) runs of a representative case?<br><b>Remarks:</b> The SOC-dependent EP-BOLFI estimations were performed only twice since they already encompass 170 individual runs that state their mean, standard deviation and confidence interval directly.                                                                                                                              | Y            |
| 3                                                                                                                                                                            | If data-driven calculations are performed (e.g., machine learning), did you specify dataset origin, the rationale behind choosing it, what information it contains, and the specific portion of it being utilized? Have you described the thought process for choosing a specific modeling paradigm?<br><b>Remarks:</b>                                                                                                                                                                                                                                                                                             | Y            |
| 4                                                                                                                                                                            | Have you discussed all sources of potential uncertainty, variability, and errors in the modeling results and their impact on quantitative results and qualitative trends? Have you discussed the sensitivity of modeling (and numerical) inputs such as material properties, time step, domain size, neural network architecture, etc. where they are variable or uncertain?<br><b>Remarks:</b>                                                                                                                                                                                                                     | Y            |
| 5                                                                                                                                                                            | Have you sufficiently discussed new or not widely familiar terminology and descriptors for clarity? Did you use these terms in their appropriate context to avoid misinterpretation? Enumerate these terms in the “Remarks”.<br><b>Remarks:</b> All electrochemical terminology is assumed to be common knowledge among battery researchers, ambiguous terminology was properly given context, and acronyms are expanded at least once. The stochastic content requires at least an undergraduate background in mathematical statistics. But the published code allows for reproducibility without said background. | Y            |
